# Supplementary material for: CubeSLAM: Monocular 3D Object SLAM
Source: arXiv:1806.00557 source file (2019-04-05)
Supplement: Supplementary file 1 [file supplementary.tex]

\section{More object detection}
Fig \ref{fig:sun rgbd more examples} and Fig \ref{fig:kitti more examples} shows more single image 3D object detection result on SUN RGBD and KITTI dataset.

\iffalse
\begin{figure*}[ht]
  \centering
   \includegraphics[scale=0.44]{03.pdf}
   \includegraphics[scale=0.44]{04.pdf}   
   \includegraphics[scale=0.44]{06.pdf}
   \includegraphics[scale=0.44]{08.pdf}
   \includegraphics[scale=0.44]{09.pdf}
   \includegraphics[scale=0.44]{10.pdf}
   \caption{
   Object SLAM result on more KITTI sequences. Note that no ground plane assumption and loop closure is applied here. Red is ground truth. Blue is our object SLAM. Green is ORB point SLAM. Objects can reduce monocular scale drift and improve pose estimation accuracy.
   }
   \label{fig:more kitti odom result}
\end{figure*}
\fi

\begin{figure*}
  \centering
   \includegraphics[scale=0.185]{sun_rgbd_object_combined_img_04.png}
   \includegraphics[scale=0.185]{sun_rgbd_object_combined_img_08.png}
   \caption{More 3D object detection examples in SUN RGBD evaluation dataset (Single View). The top view shows the predicted cuboid (blue) and ground truth matched object (red).}
   \label{fig:sun rgbd more examples}
\end{figure*}

\begin{figure*}
  \centering
   \includegraphics[scale=0.145]{kitti_object_combined_img_04.png}
   \includegraphics[scale=0.145]{kitti_object_combined_img_08.png}
   \caption{More 3D object detection examples in KITTI evaluation dataset (Single View). The top view shows the predicted cuboid (blue) and ground truth matched object (red).}
   \label{fig:kitti more examples}
\end{figure*}
